# Supplementary material for: Green Runner: A tool for efficient model selection from model repositories
Source: arXiv:2305.16849 source file (2023-05-26)
Supplement: Supplementary file 1 [file Additional_stuff.tex]

Ranking these pre-trained models is crucial from a transfer learning perspective due to the lack of sufficient data in various domains (e.g. Object detection) and brute forcing this ranking is infeasible and computationally expensive. For instance, fine-tuning a single pre-trained model on a target dataset usually costs several GPU hours and selecting the best pre-trained models from a list of 20 models will cost several GPU days. This issue has led researchers to explore efficient approximation methods for ranking pre-trained models for transfer learning. 

Existing approaches fall into two categories: offline approximation methods\cite{} which involves estimating the performance of pre-trained models on downstream tasks without fine-tuning. These methods are based on the hypothesis that the performance of a model on a pre-trained task is indicative of the performance on the target or downstream task. Offline approximation methods  and online proxy methods\cite{}. Offline approximation methods include i) Feature-based methods: These methods extract features from models such as the number of parameters, the number of layers or the activation function used to compare and rank the models, ii) Performance-based methods: These methods use performance metrics such as F1 score, accuracy, recall to rank the pre-trained models,  iii) Distance-based methods: These methods used a distance metric to rank the models. The distance calculated can be based on the weights of the models, activation of the models or other properties. However using offline methods to perform model selection has the following drawbacks i) Fixed performance: Offline model selection methods are based on pre-trained models that have been selected based on a fixed dataset. They may not perform well on unseen data, which can limit the overall accuracy of the model, ii) Resource intensive: Offline model selection methods require significant computational resources to train and evaluate multiple models. This can be particularly challenging when working with large datasets or complex models, iii) Lack of flexibility: Offline model selection methods may not be able to adapt to changing data distributions or new use cases. This can limit the overall utility of the model in real-world scenarios.

% METHOD:

Model selection is the process of choosing the best model from a set of candidate models to make accurate predictions on new data. The naive approach to solve this problem is to evaluate each candidate model on a validation dataset and select the model with the best performance, However, the problem with the naive approach is scalability. The process becomes computationally expensive and time-consuming considering the permutations (p) when there are (M) candidate  models, for the task (T) to be evaluated on dataset  (D).

In this research, our objective is to optimise the selection process, by modelling the selection approach as a multi-armed bandit problem (MAB) to investigate if we can reduce the number of data points \textbf{(Budget (B))} required from a validation set and reduce the selection time to identify the best-performing  candidate models.

\subsection{Experiment Data Collection:}
To begin our experiments have to choose a set of candidate models for an ML task. For the simplicity of the experiment, we decided to choose the task of \textit{Classification}. ML Classification is the process of categorising data into discreet classes or categories. The approach is widely used in real-world systems for spam detection, autonomous driving and traffic modelling with well-defined metrics. Metrics such as accuracy, precision, and recall, provide a quantitative measure of how well a machine learning model is performing which can be used to compare different models and select the best model. With the advantage of being well-defined and well-researched, there are many different algorithms and techniques for solving the classification problem. This feature allows us to experiment with the performance of different models and techniques for our experiment.
\subsubsection{Selection of Candidate Models:}
To perform our experiments we chose classification models from PyTorch Hub. The rationale for choosing PyTorch  Hub is that it is a widely used open-source framework for developing machine learning applications. Furthermore, The PyTorch Hub provides the official implementation of machine learning models with documentation and research papers for the models. As compared to third-party model repositories where users can upload finetuned or modified versions of machine learning models which can cause discrepancies in the performance and may lack documentation for their implementation, and training process and require additional dependencies to execute, these problems can be avoided by using official implementations available on the framework. The tools provided by the framework allow us to debug the models if there are any faults during the experiment. Additionally, the framework hosts a total of 79 image classification models. All the models are trained and evaluated on the benchmark dataset ImageNet which allows for consistency during our experiments.

\subsubsection{Dataset Selection:}
For the experiment, we utilised two datasets to collect the metrics from the candidate models. In the experiment first wanted to identify how the models performed on the benchmark dataset that the models we trained on which we call the \textit{source data set}. Second, we wanted to identify the performance of the model on unseen data which we call the \textit{target data set}. For the source dataset, we decided to use the ImageNet 1K dataset \cite{}. ImageNet1k is a large-scale visual recognition dataset with over 1.4 million labelled images in 1000 different object categories. In particular, for this experiment, we have used the image net ILSVRC 2012 version. The ILSVRC 2012 is the benchmark for image classification tasks and was used as a standard evaluation metric for deep-learning models such as AlexNet, CGG, ResNet and Inception models.

To simulate the performance of the model in a real-world setting we decided to use the ObjectNet \cite{} dataset as the target dataset. The dataset contains over 50000 images categorized in over 300 object categories. To simulate real-world characteristics of data the images in the dataset are often partially obscured, poorly lit or surrounded by clutter. In addition, the dataset includes objects from different viewpoints and scales making it difficult to recognise objects in realistic scenarios.
The advantage of using ObjectNet is that the data set contains 113 matching classes to ImageNet1k. This allows us to use the images belonging to the 113 matching classes with our candidate models without having to retrain or modify the models.

\subsubsection{Identifying Ground-Truth Models:}
For the purpose of the model selection experiment, we first needed to identify which were the best-performing ground-truth models for the target data and what is the performance degradation as compared to the performance on the source data. For collecting this information we followed the study design in \autoref{fig:gt_models}
\begin{figure}[h]
    \centering
    \includegraphics[width=\linewidth]{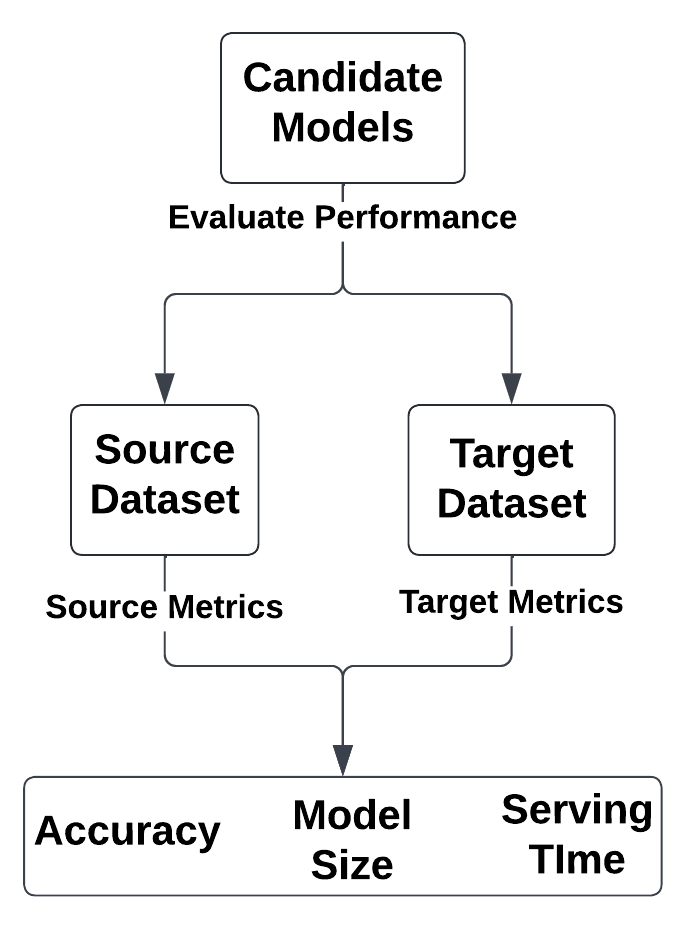}
    \caption{Study design to collect metrics which identifies the ground-truth models}
    \label{fig:gt_models}
\end{figure}

To collect the metrics which were the Top 1 per cent class accuracy for source and target dataset, Model size on disk and serving time for the models we used 3000 images from both the source dataset and images from the 113 matching classes from the target dataset to calculate the accuracy of the models, size on disk and the average serving time per image. The experiments were conducted on a system with a 2.6 GHz 6-Core Intel i7 processor with 32 Gigabytes of ram at 2667 Mhz with no additional services running in the background. Examining the results we identified the best-performing models on the source and target datasets respectively. The top 3 best performing models on the source and target data are presented in the table \autoref{}.
